# Supplementary material for: SP-ViT: Learning 2D Spatial Priors for Vision Transformers
Source: arXiv:2206.07662 source file (2022-06-15)
Supplement: Supplementary file 1 [file Appendix.pdf]

# Appendix

Anonymous CVPR submission

Paper ID 5881

## A. More Experiment Details

We show in Tab. 1 the default hyperparameters for training our SP-ViT on ImageNet-1K based on DeiT and LV-ViT respectively. All hyperparameter settings follow the baselines' except that for DeiT-based SP-ViTs we adopt a smaller learning rate.

| Base Config. | DeiT | LV-ViT |
|---|---|---|
| Supervision | Standard | Token labeling |
| SP-SA layers | 10 | 10 |
| Epoch | 300 | 300 |
| Optimizer | AdamW | AdamW |
| Batch size | 1024 | 1024 |
| LR | $2.5e-4 \cdot \frac{\text{batch size}}{512}$ | $1e-3 \cdot \frac{\text{batch size}}{640}$ |
| LR decay | cosine | cosine |
| Weight decay | 0.05 | 0.05 |
| Warmup epochs | 5 | 5 |
| Label smoothing $\epsilon$ | 0.1 | 0.1 |
| Stoch. Depth | 0.1 | 0.1 |
| Repeated Aug | ✓ | - |
| RandAug | 9/0.5 | 9/0.5 |
| Mixup prob. | 0.8 | - |
| Erasing prob. | 0.25 | 0.25 |

Table 1. Default hyperparameters for our SP-ViTs on ImageNet-1K.

## B. Python implementation

We also list our Pytorch implementation of SP-SA in Listing 1. SP-SA can be easily integrated into any existing vision transformer models by directly replacing a number of SA layers. Calculating the relative coordinates to query patches is trival, so this part of code is not included for simplicity. Note that the insertion of classification token should be moved after SP-SA layers, as mentioned in the main text.

## C. More Visualization

We provide more examples of learned Spatial Priors (SP) by our SP-ViT based on DeiT-Small and trained on ImageNet-1K in Fig. 1 and Fig. 2.

**Listing 1** SP-SA `SP-SA.py`

```
import torch
from torch import nn

class SP_SA(nn.Module):
    def __init__(self, dim, num_heads=8, qk_scale=None, attn_drop=0., proj_drop=0., rel_indices=None
        , **kwargs):
        super().__init__()
        self.num_heads = num_heads
        self.dim = dim
        head_dim = dim // num_heads
        self.scale = qk_scale or head_dim ** -0.5
        self.v = nn.Linear(dim, dim, bias=False)
        self.qk = nn.Linear(dim, dim * 2, bias=False)
        self.w1 = nn.Linear(2, dim, bias=True)
        self.w2 = nn.Parameter(torch.zeros(dim, 1))
        self.b2 = nn.Parameter(torch.ones(num_heads))

        self.attn_drop = nn.Dropout(attn_drop)
        self.proj = nn.Linear(dim, dim)
        self.proj_drop = nn.Dropout(proj_drop)
        self.act = nn.ReLU()
        self.rel_indices = rel_indices

    def forward(self, x):
        B, N, C = x.shape
        attn = self.get_attention(x)

        v = self.v(x).reshape(B, N, self.num_heads, C // self.num_heads).permute(0, 2, 1, 3)
        x = (attn @ v).transpose(1, 2).reshape(B, N, C)
        x = self.proj(x)
        x = self.proj_drop(x)
        return x

    def get_attention(self, x):
        B, N, C = x.shape

        # Calculating Patch Score
        qk = self.qk(x).reshape(B, N, 2, self.num_heads, C // self.num_heads).permute(2, 0, 3, 1, 4)
        q, k = qk[0], qk[1]
        patch_score = (q @ k.transpose(-2, -1)) * self.scale

        # Calculating Spatial Prior
        sp_hidden = self.w1(self.rel_indices).view(1, N, N, self.num_heads, self.dim // self.
            num_heads)
        sp = torch.einsum('nm,hijnm->hijn', (self.w2.view(self.num_heads, -1), self.act(sp_hidden)))
             + self.b2
        sp = sp.repeat(B, 1, 1, 1)

        enhanced_attention = (patch_score * sp.permute(0, 3, 1, 2)).softmax(dim=-1)
        attn = self.attn_drop(enhanced_attention)
        return attn
```

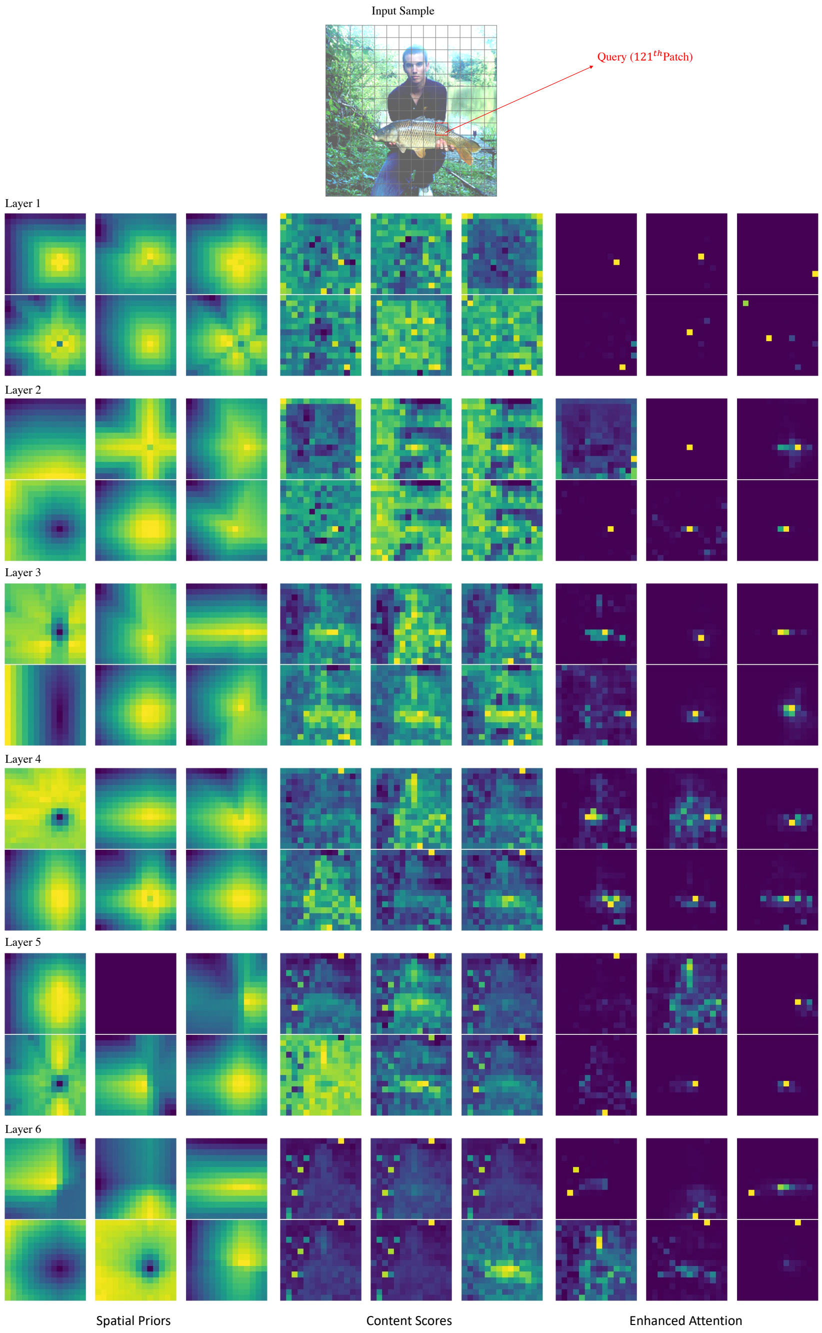


Figure 1. More Visualization of the learned 2D SPs, content scores and the enhanced attention of layer 1-6 for the $121^{th}$ query patch.

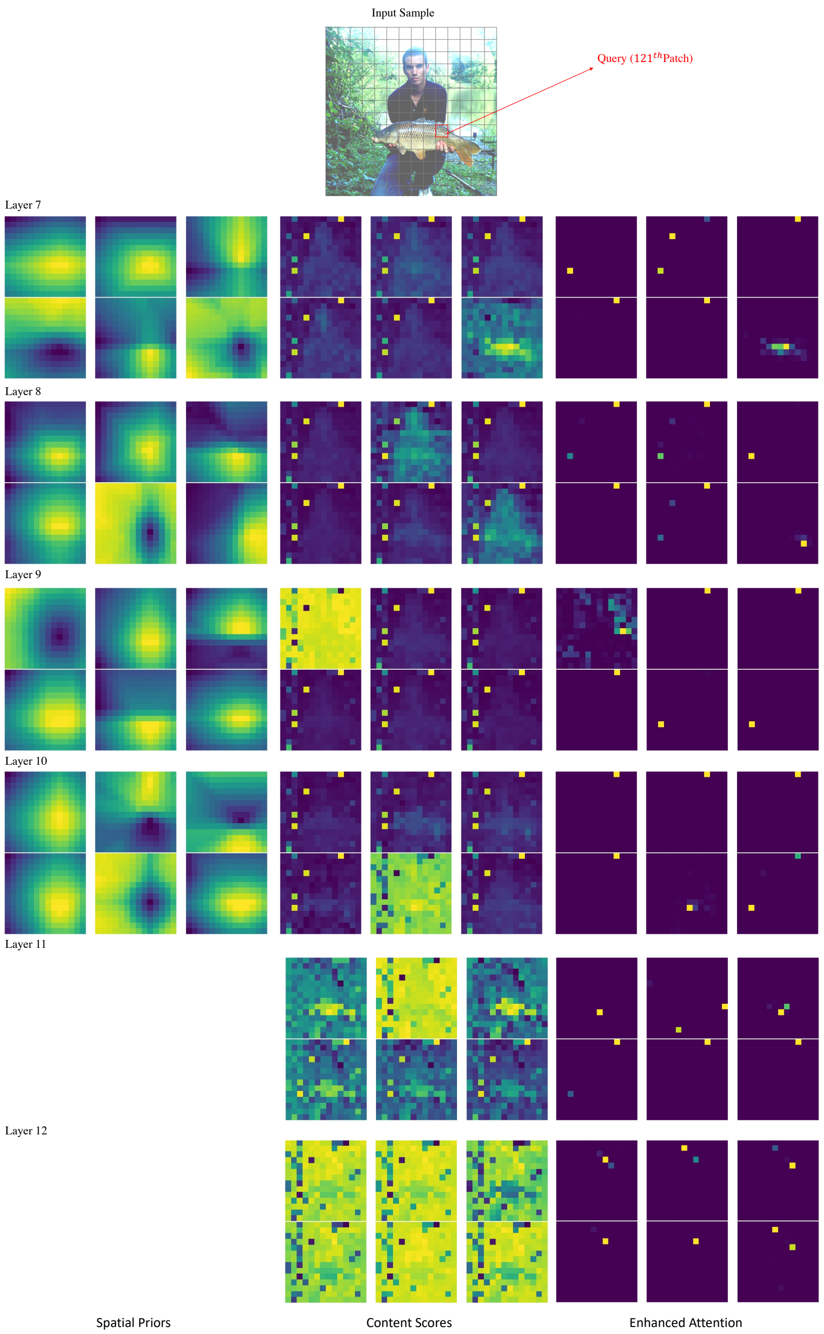


Figure 2. More Visualization of the learned 2D SPs, content scores and the enhanced attention of layer 7-12 for the $121^{th}$ query patch. Note that layer 11 and 12 are vanilla SA layers, thus no spatial priors are existed.
